# Supplementary material for: Portfolio Optimization under Nonlinear Utility
Source: arXiv:1504.03931 source file (2015-04-15)
Supplement: Supplementary file 1 [file appendix02.tex]

\section{Pathwise Differentiability of Quadratic BSDE: A Generalisation}\label{sec:annex1}
The question about the differentiability of BSDE --- in the standard sense as well as in the Malliavin one --- raised very early in \cite{karoui01} for instance.
The growing interest for quadratic BSDE and the need of some results about the regularity of BSDE-flows brought several generalization of this differentiability results, see \cite{imkeller01}, \cite{a08}  or \cite{briand01}.

For our purpose, these results suffers some shortcomings.
In \cite{imkeller01} among plenty other assumptions will be assumed that the generator of the BSDE is behaving in $z$ as a constant times $\norm{z}^2$.
In our case, see \ref{eq:BSDEentropieclassic}, this constant depends on $\gamma$.
Moreover, the generator has a specific shape, which does not completely fit in our context.
We aim generally at having a generator which is H\"older continuous of order $2$ in $z$ and $1$ in $y$.

In \cite{briand01} the generator of the BSDE possesses the wished general shape, but does not depends separately on the $\gamma$ but on a forward diffusion process starting at $\gamma$.
Moreover, the results do not entail some a-priori estimates for the quadratic BSDE as well as for the linear BSDE with Lipschitz random constant, which are crucial to prove the H\"older continuity of the derivative of the solution with respect to the parameter, which in turns is necessary to get some pathwise differentiability.

The goal of this annex is then to simply mix both results to obtain the necessary assumption on the driver needed in \ref{sec01}. Indeed, this will consist in a from times to times stupid re-writing of the results obtained in \cite{imkeller01} or \cite{briand01} to obtain this slightly generalized differentiability result, but besides this we obtain a result about the H\"older continuity of the derivative w.r.t. to the H\"older continuity of the driver. 

In the following we are considering a parameter depending BSDE of the type:
\begin{equation}
	Y_t\left( \gamma \right)=X\left( \gamma \right)+\int_{t}^{T}f\left( t,\gamma,Y_s\left( \gamma \right),Z_{s}\left( \gamma \right) \right)ds -\int_{t}^{T}Z_{s}\left( \gamma \right)\bullet dB_{s},
	\label{eq:ap01:BSDE01}
\end{equation}
where the generator and terminal conditions are subject to the following sets of conditions. For existence and uniqueness of \eqref{eq:ap01:BSDE01} we need:
\begin{enumerate}[label=(E-\roman*)]
	\item $f: \Omega\times \left[ 0,T \right]\times \mathcal{O}\times \R \times \R^d \rightarrow \R$ is an adapted measurable function, where $\mathcal{O}$ is an open set of $\R^n$;
	\item $|f(s,\gamma,y,z|\leq C(1+|y|+|z|^2)$;
	\item $X(\gamma)$ is bounded.
\end{enumerate}
For differentiability with respect to $\gamma$ we assume, there exists $C\geq 0$ and $\alpha_{K}\in(0,1)$ such that
\begin{enumerate}[label=(D-\roman*)]
	\item $f\left( s,\cdot,\cdot,\cdot \right)$ is $C^{1,1,1}\left( \mathcal{O}\times \R \times \R^d ; \R\right)$;
	\item $\gamma \rightarrow X\left( \gamma \right)$ is $C^1\left( \R^n;\Lp{\infty} \right)$;
	\item $|\partial_{\gamma}X(\gamma)| \leq C(1+|\gamma|^n)$;
	\item $|\partial_{\gamma}f\left( s,\gamma, y,z\right)|\leq C(1+|\gamma|^n + |z|^2)$;
	\item $|\partial_{z}f\left( s,\gamma, y,z\right)|\leq C(1+|z|)$;
	\item $|\partial_{y}f\left( s,\gamma, y,z\right)|\leq C(1+|z|)^{2\alpha_{K}}$.
\end{enumerate}	
For pathwise differentiability with respect to $\gamma$ we further need that 
\begin{enumerate}[label=(PD a-\roman*)]
	\item $|f(s,\gamma,y,z)-f(s,\gamma,y,z')|\leq K(1+|z|+|z'|)|z-z'|$, a.s.;
	\item $|f(s,\gamma,y',z)-f(s,\gamma,y',z)|\leq K|y-y'|$, a.s.
\end{enumerate}
And also
\begin{enumerate}[label=(PD b-0)]
	\item $|f(s,\gamma,y,z)-f(s,\gamma',y,z)|\leq C|\gamma-\gamma'|^{\alpha}$, a.s.
\end{enumerate}
In addition we will impose the following conditions. There exists $\alpha \geq 0$, and for any compact $K \subset \mathcal{O}$, there exists $C_K\geq 0$ and $\alpha_K \in \left] 0,1 \right[$ such that over $K$ holds:
\begin{enumerate}[label=(PD b-\roman*)]
	\item $|X\left( \gamma \right)-X\left( \gamma' \right)|\leq C|\gamma-\gamma'|^\alpha$;
	\item $\sup_{\gamma \in K}\norm{\partial_{\gamma}X\left( \gamma \right)}_{\infty}\leq M$;
	\item $|\partial_{\gamma}X\left( \gamma \right)-\partial_{\gamma}X\left( \gamma' \right)|\leq C|\gamma-\gamma'|^\alpha$;
	\item $\abs{\partial_{\gamma}f\left( s,\gamma, y,z\right)-\partial_{\gamma}f\left( s,\gamma', y',z'\right)}\leq C\left(\norm{\gamma-\gamma'}^\alpha+\norm{z-z'}^2 \right)$;
	\item $\abs{\partial_{y}f\left( s,\gamma,y,z \right)-\partial_{y}f\left( s,\gamma',y',z' \right)}\leq C\left( \norm{z-z'}^{2\alpha_K}+\norm{\gamma-\gamma'}^\alpha\right)$;
	\item $\abs{\partial_{z}f\left( s,\gamma,y,z \right)-\partial_{z}f\left( s,\gamma',y',z' \right)}\leq C\left( \norm{z-z'}+\norm{\gamma-\gamma'}^\alpha\right)$;
	\item $\alpha>0$ .
\end{enumerate}

The generalization we aim at showing is the subject of the following theorem.
\begin{thm}\label{thm:differentiabilityBSDE}
	Under hypothesis (E-i) to (E-iii) and (D-i) to (D-vi), there exists a solution $\left( Y\left( \gamma \right),Z\left( \gamma \right) \right)$ to \ref{eq:ap01:BSDE01}, and the map $\gamma \mapsto \left( Y\left( \gamma \right),Z\left( \gamma \right) \right)$ is in $C^1\left( \mathcal{S}^p \times \mathcal{M}^p \right)\subset C^1\left( \mathcal{M}^p \times \mathcal{M}^p \right)$.
	
	Moreover, for every $\gamma$, the derivative processes $\left(\nabla_\gamma Y\left( \gamma \right),\nabla_{\gamma} Z\left( \gamma \right)\right)$ are solutions of the following linear BSDE:
	\begin{equation}
		\begin{split}
			\nabla_{\gamma}Y_{t}\left( \gamma \right)=\partial_{\gamma}X\left( \gamma \right)&+\int_{t}^{T}\partial_{\gamma}f\Big( s,\gamma,Y_{s}\left( \gamma \right),Z_{s}\left( \gamma \right)\Big)\;ds+\int_{t}^T \partial_{y}f\Big( s,\gamma,Y_{s}\left( \gamma \right),Z_{s}\left( \gamma \right) \Big)\nabla_{\gamma}Y_{s}\left( \gamma \right)\;ds\\
			&+ \int_{t}^{T}\partial_{z}f\Big( s,\gamma,Y_{s}\left( \gamma \right),Z_{s}\left( \gamma \right)\Big)\nabla_{\gamma}Z_{s}\left( \gamma \right)\;ds-\int_{t}^{T}\nabla_{\gamma}Z_{s}\left( \gamma \right)\bullet dB_{s}
	\end{split}
		\label{eq:ap01:BSDEdiff01}
	\end{equation}
	And there exists $C_p$ such that:
	\begin{equation}
		\norm{\nabla_{\gamma}Y\left( \gamma \right)}_{\mathcal{S}^p}+\norm{\nabla_{\gamma}Z\left( \gamma \right)}_{\mathcal{M}^p}\leq C_{p}\left( 1+\norm{\gamma} \right)^\alpha
		\label{eq:ap:diffapp01}
	\end{equation}
	Further, under (PD a-i) to (PD a-ii) and (PD b-i) to (PD b-vii), $\gamma \mapsto \partial_{\gamma}Y\left( \gamma \right)$ from $\R^n$ to $\mathcal{M}^p$ is H\"older continuous of order $\alpha$ for each $p>2$, and it is possible to find a version of $Y\left( \gamma \right)$ which is path wise continuously differentiable and has as derivative $\nabla_\gamma Y\left( \gamma \right)$.
\end{thm}

\begin{rem}\label{rem:pd:entropic}
The conditions required for the above theorem to hold are not sharp. A study of the proof shows that some of the H\"older type conditions placed on the generator can be replaced by certain integrability conditions. For example condition (PD b-iv) could be replaced by 
\begin{equation*}
E\left[\left(\int_0^T \abs{\partial_{\gamma}f\left( s,\gamma, Y_s(\gamma),Z_s(\gamma)\right)-\partial_{\gamma}f\left( s,\gamma', Y_s(\gamma'),Z_s(\gamma')\right)}ds\right)^q \right]\leq C(|\gamma-\gamma'|^{\alpha})^q,
\end{equation*}
for a certain $q>1$. In order to verify such inequalities one usually employs results on the $\mathcal{M}^p$ boundedness of $Z$ and a priori estimates for quadratic BSDEs. For more details in a specific situation, namely the generator $f$ considered in Section ??, see Corollary \ref{cor:pd:entropic}.
\end{rem}

The strategy used to prove this theorem relies on three results\footnote{Strategy applied in \cite{imkeller01} and \cite{a08}}:
\begin{enumerate}
	\item Moment estimates for linear BSDE with random Lipschitz constant.
		This concerns the Proposition \ref{prop:momentestimates} which has been already proved in \cite{imkeller01}, Theorem 3.1.

		These moment estimates allows us to solve the part about the differentiability in the theorem \ref{thm:differentiabilityBSDE}.
	
	\item A-priori estimates for linear BSDE with random Lipschitz constant: This is the subject of the Proposition \ref{prop:apriorilinearestimates} which also has been proved in \cite{imkeller01}, Theorem 4.1.
	\item A-priori estimates for quadratic BSDE: Proposition \ref{prop:aprioriestimates} is dedicated to these estimates.
		These a-priori estimates together with the preceding ones are the key arguments to crack the H\"older continuity of the derivative in theorem \ref{thm:differentiabilityBSDE}
\end{enumerate}

\subsection{Linear BSDEs and a priori estimates for quadratic BSDEs}
In this section we collect some material on linear BSDEs with random Lipschitz constants and we cite a result of \cite{a08} concerning a priori estimates for quadratic BSDEs.

When we speak about linear BSDE --- depending on a parameter $\gamma$ --- with random Lipschitz constant we mean:
\begin{equation}
	U_t\left( \gamma \right)=X\left(\gamma  \right)+\int_{t}^{T}\bigg(A_s\left( \gamma \right)+D_s\left( \gamma \right) U_s\left( \gamma \right)+C_s\left( \gamma \right)\bullet V_s\left( \gamma \right) \bigg)ds-\int_{t}^{T}V_{s}\left( \gamma \right) \bullet dB_s
	\label{eq:LBSDE}
\end{equation}

Consider the following set of assumption:
\begin{enumerate}%[(\textnormal{A}-i)]
	\item $X\left( \gamma \right) \in \Lp{\infty}$
	\item $C\left( \gamma \right)$ is a predictable $\R^d$ value process, integrable w.r.t. $B$ and such that $\int_{0}^{\cdot}C\bullet dB$ is a BMO-martingale\footnote{For definition, notations and results about BMO martingales we refer to \cite{kazamaki01} by \textsc{Kazamaki N.}}.
	\item $D\left( \gamma \right)$ is a measurable adapted process essentially bounded by some constant $M\left( \gamma \right)$.
	\item $A\left( \gamma \right)$ is a measurable adapted process such that for all $p\geq 1$:
		$$E\left[ \left(\int_{0}^{T}\abs{A_s}ds\right)^p \right]<\infty$$
	\item Both:
		$$\left( \int_{0}^{T} \abs{U_s\left( \gamma \right)}^2\norm{V_s}^2 ds\right)^{\frac{1}{2}}\qquad \text{and}\qquad \int_{0}^{T} \abs{U_s\left( \gamma \right) A_s\left( \gamma \right)}ds$$
		are $p$-integrable for all $p\geq 1$.
\end{enumerate}
For the following proposition, because it concerns only one BSDE, we drop the reference to $\gamma$ for notational convenience.
\begin{prop}\label{prop:momentestimates}
Assume that (A-i) to (A-v) are satisfied.
Let $p>1$ and $r>1$ such that $\mathcal{E}\left(\int_0^\cdot C \bullet dB\right)_T$ is in $\Lp{r}$. Then there exists a constant $C$ depending only on $p,T$ the essential supremum of $D$ and the BMO-norm of $\int_{0}^{\cdot}C\bullet dB$ such that for the conjugate exponent $q$ of $r$ we have:
\begin{equation}
	E\left[ \sup_{t \in \left[ 0,T \right]}\abs{U_t}^{2p} \right]+E\left[ \left( \int_{0}^{T}\norm{V_{s}}^2 ds \right)^p \right] \leq C E\left[ \abs{X}^{2pq^2}+\left( \int_{0}^{T}\abs{A_s}ds \right)^{2pq^2} \right]^{\frac{1}{q^2}}
	\label{eq:momentestimates01}
\end{equation}
Moreover:
\begin{equation}
	E\left[ \int_{0}^{T}\abs{U_s}^{2}ds \right]+E\left[  \int_{0}^{T}\norm{V_{s}}^2 ds \right] \leq C E\left[ \abs{X}^{2q^2}+\left( \int_{0}^{T}\abs{A_s}ds \right)^{2q^2} \right]^{\frac{1}{q^2}}
	\label{eq:momentestimates02}
\end{equation}
\end{prop}
The proof of this proposition can be founded in \cite{imkeller01} page 7-10.

For the following proposition, we consider the linear BSDE \ref{eq:LBSDE} for two parameters, $\gamma,\gamma'$ fulfilling the assumption (A-i) to (A-v).

In order to facilitate the notation, we drop the reference to $\gamma$ and $\gamma'$ to replace it only by a $'$ for the elements of the second linear BSDE.
Throughout let $\delta U=U-U'$, $\delta V= V-V'$ and so on for $\delta X$, $\delta A$, $\delta D$ and $\delta C$.
\begin{prop}\label{prop:apriorilinearestimates}
	Suppose that we have for all $\beta\geq 1$, $\int_{0}^{T}\abs{\delta U_s}^2\norm{\delta V_s}^2 ds \in \Lp{r}$ and $\int_{0}^T \abs{\delta U_s}\abs{\delta A_s} ds \in \Lp{r}$.
	For $p >1$ and $r >1 1$ such that $\mathcal{E}\left( \int_{0}^{\cdot}C'\bullet dB \right)_T \in \Lp{r}$.
	Then, there exists a constant $C>0$ depending only on $p$, $t$, the essential supremum of $D$ and the BMO-norm of $\int_{0}^{\cdot}C'\bullet dB$, such that with the conjugate $q$ of $r$ we have:
	\begin{equation}
		\begin{split}
			E&\left[ \sup_{t \in \left[ 0,T \right]}\abs{\delta U_t}^{2p} \right]+E\left[ \left( \int_{0}^{T}\norm{\delta V_s}^2 ds \right)^p \right]\\
			&\qquad\leq C\Bigg\{E\left[ \abs{\delta X}^{2pq^2}+\left( \int_{0}^{T} \abs{\delta A_s+U_s' \delta D_s}ds \right)^{2pq^2} \right]^{\frac{1}{q^2}}\\
			&\qquad \qquad \qquad +E\left[ \abs{X}^{2pq^2} +\left( \int_{0}^{T}\abs{A_s}ds \right)^{2pq^2} \right]^{\frac{1}{2q^2}}E\left[ \left( \int_{0}^{T}\norm{\delta C_s}^2 ds\right)^{2pq^2} \right]^{\frac{1}{2q^2}}\Bigg\}
		\end{split}
		\label{eq:apriorilinearestimates}
	\end{equation}
\end{prop}
The proof of this proposition can be founded in \cite{imkeller01} page 10-13.

We are looking now for some a-priori estimates for quadratic BSDE of the form \ref{eq:ap01:BSDE01}.
We consider two of these BSDE \ref{eq:ap01:BSDE01} for two different parameters $\gamma$ and $\gamma'$.
As before we drop the reference to $\gamma$ or $\gamma'$ to keep the notation only with the $'$, i.e. for instance, $f'\left( t,y,z \right)=f\left( t,\gamma',y,z \right)$, and the same for the notation with $\delta$.

Note first that, in reason of the boundedness of $X$ and $X'$, both $\int_{0}^{\cdot}Z\bullet dB$ and $\int_{0}^\cdot Z'\bullet dB$ are BMO-martingales.
\begin{prop}\label{prop:aprioriestimates}
	Assume that (E-i) to (E-iii) and (PD a-i) to (PD a-ii) hold for both BSDEs.
	Furthermore, suppose that for all $\beta \geq 1$, we have $\int_0^T \delta f\left( s,Y'_s,Z_s' \right)ds \in \Lp{\beta}$.
	For all $p\geq 1$ there exists constants $q \in (1,\infty)$ and $C\in \R_+$, depending only on $p$, $K$, $T$ and $||X||_{\infty}$ such that
	\begin{equation}
		\begin{split}
			E\left[ \sup_{t \in \left[ 0,T \right]}\abs{\delta Y_t}^{2p} \right]+E\left[ \left( \int_{0}^{T}\norm{\delta Z_s}^2 ds \right)^{p} \right]\leq CE\left[ \abs{\delta X}^{2pq^2}+ \left( \int_{0}^{T}\abs{\delta f \left( s,Y'_s,Z_s' \right)}ds \right)^{2pq^2} \right]^{\frac{1}{q^2}}	.	
		\end{split}
		\label{eq:aprioriestimates01}
	\end{equation}
\end{prop}
The proof of this proposition can be found in \cite{a08}, page 18 ff.

\subsection{Differentiability of \eqref{eq:ap01:BSDE01}}

Let us now come back to theorem \ref{thm:differentiabilityBSDE}.
The first part of its proof is an easy adaptation of the proof of  Proposition 12 in \cite{briand01} and will be given in the following Lemma.
The difference here, is that we do not consider a BSDE depending on a forward SDE, but a driver and a terminal condition directly depending smoothly on a parameter in the spirit of \cite{imkeller01}.
\begin{lem}
Under (E-i) to (E-iii) and (D-i) to (D-vi) the map $\gamma \mapsto (Y(\gamma),Z(\gamma))$ belongs to $C^1\left( \mathcal{S}^p \times \mathcal{M}^p \right)$. Moreover the derivative process $(\nabla_{\gamma}Y,\nabla_{\gamma}Z)$ solves the BSDE \eqref{eq:ap01:BSDEdiff01} and there exists $C_{p}>0$ such that Estimate \eqref{eq:ap:diffapp01} holds.

\end{lem}
\begin{proof}
	For all $t \in \left[ 0,T \right]$, the continuity of the map $\gamma \mapsto \left( Y_t\left( \gamma \right),Z_{t}\left( \gamma \right) \right)$ is already contained in Kobylanski's stability theorem in \cite{kobylanski01}. 
	
	We fix $\gamma \in \mathcal{O}$ and set $\varepsilon >0$ such that $B\left( \gamma,\varepsilon \right)\subset \mathcal{O}$.
	$\bar{B}\left( \gamma,\varepsilon \right)$ is the compact $K$ in the hypothesis there before.

	Under (E-i) to (E-iii), there exists a unique solution to the BSDE \eqref{eq:ap01:BSDE01}, see \cite{kobylanski01}.
	Moreover, by \cite{briand01}, Equation (12), for each $\gamma$ there exists a constant $C$ such that:
	\begin{equation}
		\norm{\sup_{t \in \left[ 0,T \right]} \abs{Y_{t}\left( \gamma \right)}}_{\infty}+\norm{\int_{0}^{\cdot}Z_{s}\left( \gamma \right)\bullet dB_{s}}_{BMO_2}\leq C.
		\label{eq:cestmaintenant}
	\end{equation}
	The boundedness of $Y$ is due to \cite{lepeltier01} and the BMO norm estimation of $Z$ is completed by computation through Ito Formula with $(e^{2\alpha x}-2\alpha x-1)/(2\alpha^2)$ applied between $\tau$ and $T$ on $Y$ for any stopping time $\tau<T$ as stated in \cite{briand01}.
	In particular, see \cite{briand01}, Equation (13), for each $p \geq 1$
	\begin{equation}
		\norm{\left( \int_{0}^{T}\norm{Z_{s}}^2 ds \right)^{\frac{1}{2}}}_{p}\leq C_{p}.
		\label{eq:ap:inter01}
	\end{equation}
From this and from (D-iii) and (D-iv) we deduce for all $p>1$:
	\begin{equation*}
		\norm{\abs{\partial_{\gamma}X\left( \gamma \right)}+\int_{0}^{T}\abs{\partial_{\gamma}f\left( s,\gamma,Y_{s}\left( \gamma \right),Z_{s}\left( \gamma \right) \right)}ds}_{p}\leq C_{p}\left( 1+\norm{\gamma} \right)^m.
		\label{}
	\end{equation*}
	It means that the generator of BSDE \eqref{eq:ap01:BSDEdiff01} fulfills the hypothesis of Theorem 10 in \cite{briand01}, therefore has a unique solution in $\mathcal{S}^p\times \mathcal{M}^p$. Moreover Corollary 9 in \cite{briand01} and \eqref{eq:ap:inter01} imply that \eqref{eq:ap:diffapp01} holds.

	For $h \in \left] 0,\varepsilon \right[$, we define $U^{h}=\frac{Y\left( \gamma +h\right)-Y\left( \gamma \right)}{h}-\nabla_{\gamma}Y\left( \gamma \right)$ and $V^{h}=\frac{Z\left( \gamma +h\right)-Z\left( \gamma \right)}{h}-\nabla_{\gamma}Z\left( \gamma \right)$ which solve the following BSDE:
	\begin{equation*}
		\begin{split}
			U_t^h&=\frac{X\left( \gamma +h \right)-X\left( \gamma \right)}{h}-\partial_{\gamma} X\left( \gamma \right)-\int_{t}^{T}V_{s}^\varepsilon \bullet dB_{s}\\
			&\quad +\int_{t}^{T}\frac{f\left( s,\gamma+h,Y_s\left( \gamma+h \right),Z_s\left( \gamma+h \right) \right)-f\left( s,\gamma,Y_s\left( \gamma \right),Z_s\left( \gamma \right) \right)}{h}ds\\
			&\quad -\int_{t}^{T}\partial_{\gamma}f\Big( s,\gamma,Y_{s}\left( \gamma \right),Z_{s}\left( \gamma \right)\Big)\;ds -\int_{t}^T \partial_{y}f\Big( s,\gamma,Y_{s}\left( \gamma \right),Z_{s}\left( \gamma \right) \Big)\nabla_{\gamma}Y_{s}\left( \gamma \right)\;ds\\
			&\quad - \int_{t}^{T}\partial_{z}f\Big( s,\gamma,Y_{s}\left( \gamma \right),Z_{s}\left( \gamma \right)\Big)\nabla_{\gamma}Z_{s}\left( \gamma \right)\;ds\\
			&=\frac{X\left( \gamma +h \right)-X\left( \gamma \right)}{h}-\partial_{\gamma} X\left( \gamma \right)-\int_{t}^{T}V_{s}^\varepsilon \bullet dB_{s}\\
			&\quad + \int_{t}^{T}\left(A^h_{s}U_{s}^{h}+D^h_s V_s^h\right) ds+\int_{t}^{T}\left(P_s^h+Q_s^h+R_s^h\right)ds
		\end{split}
		\label{}
	\end{equation*}
Where $A,D,P,Q,R$, after remarking that
\begin{equation*}
	\begin{split}
	\frac{1}{h}&\bigg( f\Big( t,\gamma +h,Y_{t}\left( \gamma+h \right),Z_t\left( \gamma+h \right) \Big)-f\Big( t,\gamma,Y_{t}\left( \gamma \right),Z_{t}\left( \gamma \right) \Big) \bigg)\\
	&=\int_{0}^{1}\partial_{\gamma}f\left( t,\gamma+\theta h,Y_t\left( \gamma \right),Z_{t}\left( \gamma \right) \right)d\theta\\
	&+\frac{Y_t\left( \gamma+h \right)-Y_{t}\left( \gamma \right)}{h}\int_{0}^{1}\partial_{y}f\left( t,\gamma+h,Y_t\left( \gamma \right)+\theta \left(Y_t\left( \gamma+h \right)-Y_{t}\left( \gamma \right)\right),Z_{t}\left( \gamma \right) \right)d\theta\\
	&+\frac{Z_t\left( \gamma+h \right)-Z_{t}\left( \gamma \right)}{h}\int_{0}^{1}\partial_{z}f\left( t,\gamma+h,Y_t\left( \gamma+h \right),Z_t\left( \gamma \right)+\theta \left(Z_t\left( \gamma+h \right)-Z_{t}\left( \gamma \right)\right)\right)d\theta\\
\end{split}
	\label{}
\end{equation*}
are given by:
\begin{eqnarray*}
	A_t^h&=&\int_{0}^{1}\partial_{y}f\Big( t,\gamma+h,Y_t\left( \gamma \right)+\theta \left(Y_t\left( \gamma+h \right)-Y_{t}\left( \gamma \right)\right),Z_{t}\left( \gamma \right) \Big)d\theta\\
	D_t^h&=&\int_{0}^{1}\partial_{z}f\Big( t,\gamma+h,Y_t\left( \gamma+h \right),Z_t\left( \gamma \right)+\theta \left(Z_t\left( \gamma+h \right)-Z_{t}\left( \gamma \right)\right)\Big)d\theta\\
	P_t^h&=&\bigg(A_t^h-\partial_y f\Big(t,\gamma,Y_s\left( \gamma \right),Z_s\left( \gamma \right)  \Big)\bigg)\nabla_\gamma Y_{s}\left( \gamma \right)\\
	Q_t^h&=&\bigg(D_t^h-\partial_z f\Big(t,\gamma,Y_s\left( \gamma \right),Z_s\left( \gamma \right)  \Big)\bigg)\nabla_\gamma Z_{s}\left( \gamma \right)\\
	R_t^h&=&\int_{0}^{1}\partial_{\gamma}f\Big( t,\gamma+\theta h,Y_t\left( \gamma \right),Z_{t}\left( \gamma \right) \Big)d\theta-\partial_{\gamma}f\Big( t,\gamma,Y_t\left( \gamma \right),Z_{t}\left( \gamma \right) \Big)
\end{eqnarray*}
The hypothesis (D-iv) to (D-vi) yield:
\begin{eqnarray*}
	\abs{A_t^h}&\leq&C\left( 1+\norm{Z_t\left( \gamma \right)}+\norm{Z_t\left( \gamma+h \right)}\right)^{2 \alpha_K}\\
	\abs{D_t^h}&\leq&C\left( 1+\norm{Z_t\left( \gamma \right)}+\norm{Z_{t}\left( \gamma+h \right)} \right)\\
	\abs{P_t^h}&\leq&C\left( 1+\norm{Z_t\left( \gamma \right)}+\norm{Z_{t}\left( \gamma+h \right)} \right)^{2\alpha_K}\abs{\nabla_\gamma Y_t\left( \gamma \right)}\\
	\abs{Q_t^h}&\leq&C\left( 1+\norm{Z_t\left( \gamma \right)}+\norm{Z_{t}\left( \gamma+h \right)} \right)\norm{\nabla_\gamma Z_t\left( \gamma \right)}\\
	\abs{R_t^h}&\leq&C\left( 1+\norm{\gamma}+\norm{\gamma+h}+\norm{Z_t\left( \gamma \right)} \right)
\end{eqnarray*}
This, the Inequalities \eqref{eq:cestmaintenant}, \eqref{eq:ap:inter01} and the Corollary 9 in \cite{briand01} guarantee the existence of some $p>1$ such that:
\begin{equation}
	\begin{split}
	\norm{U^h}_{\mathcal{S}^p}+\norm{V^h}_{\mathcal{M}^p}&\leq C\norm{\frac{X\left( \gamma +h \right)-X\left( \gamma \right)}{h}-\partial_{\gamma} X\left( \gamma \right)}_{p+1}\\
	&\quad\qquad+C\norm{\int_{0}^{T}\Big(\abs{P_t^h}+\abs{Q_t^h}+\abs{R_t^h}\Big)dt}_{p+1}
\end{split}
	\label{eq:presquelafin}
\end{equation}
The previous inequality concerning $A,D,P,Q$ and $R$, the regularity of $X\left( \cdot \right)$ and $f$ together with Lebesgue's dominating convergence let the right hand side of \eqref{eq:presquelafin} converge to $0$, and this ends the proof of the differentiability and the fact that $\nabla_\gamma Y$ and $\nabla_{\gamma}Z$ are given by the solution of BSDE \eqref{eq:ap01:BSDE01}.
\end{proof}

It remains now to see the proof of the H\"older continuity of the derivative of the solution under hypothesis (PD-i) to (PD-vii).
To this aim, we will use the a-priori estimates properties established in Propositions \ref{prop:apriorilinearestimates} and \ref{prop:aprioriestimates}.
\begin{lem}
Suppose (E-i) to (E-iii), (D-i) to (D-vi), (PD a-i) to (PD a-ii) and (PD b-i) to (PD b-vii) hold. Then the map $\gamma \mapsto Y(\gamma)$ is pathwise differentiable.
\end{lem}
\begin{proof}
For $\gamma,\gamma' \in \mathcal{O}$, consider a compact $K\subset \mathcal{O}$ containing in its interior $\gamma$ and $\gamma'$.
The processes $\nabla_\gamma Y\left( \gamma \right)$ and $\nabla_{\gamma}Y\left( \gamma' \right)$ are solutions of linear BSDEs with random Lipschitz constants. In particular, letting $U(\gamma) = \nabla_\gamma Y\left( \gamma \right)$, we have
\begin{equation}
	U_t\left( \gamma \right)=\partial_{\gamma}X\left( \gamma \right)+\int_{t}^{T}\bigg(A_s\left( \gamma \right)+D_s\left( \gamma \right) U_s\left( \gamma \right)+C_s\left( \gamma \right)\bullet V_s\left( \gamma \right) \bigg)ds-\int_{t}^{T}V_{s}\left( \gamma \right) \bullet dB_s,
	\label{eq:ap:proof:path:LBSDE}
\end{equation}
where
\begin{equation}
\begin{split}
A_s\left( \gamma \right) &= \partial_{\gamma}f\Big( s,\gamma,Y_{s}\left( \gamma \right),Z_{s}\left( \gamma \right)\Big), \\
D_s\left( \gamma \right) &= \partial_{y}f\Big( s,\gamma,Y_{s}\left( \gamma \right),Z_{s}\left( \gamma \right) \Big),\\
C_s\left( \gamma \right) &= \partial_{z}f\Big( s,\gamma,Y_{s}\left( \gamma \right),Z_{s}\left( \gamma \right)\Big).
\end{split}
		\label{eq:ap:proof:path:01}
\end{equation}
The respective linear BSDE for $\nabla_{\gamma}Y\left( \gamma' \right)$ can be written in an analogous fashion. To simplify notation, we note everything related to $\gamma'$ with a $'$, i.e. for instance $Z\left( \gamma' \right)=Z'$ and $Z\left(\gamma \right)=Z$, and everything related to a difference between $'$ and non-$'$ with $\delta$, i.e. for instance $\delta Z=Z-Z'$.

In order to show the H\"older continuity we will estimate the difference $\delta U = U-U'=\nabla_\gamma Y\left( \gamma \right)-\nabla_{\gamma}Y\left( \gamma' \right)$ with the a priori estimate obtained in Proposition  \ref{prop:apriorilinearestimates}.

Remark that $\gamma \mapsto \norm{\int_{0}^{\cdot}\nabla_{\gamma} Z\left( \gamma \right)\bullet dB}_{BMO-2}$ is finite and continuous.
Using the reverse H\"older property in \cite{kazamaki01}, we can then find some real $r>1$ such that for all $\gamma \in K$, $\mathcal{E}_{0,T}\left( \nabla_{\gamma}Z\left( \gamma \right)\bullet dB \right)\in \Lp{r}$.
Note with $q$ the conjugate of $r$.

In the following, the $C$ denotes a constant, which may vary from line to line, but depends at most on $p$, $T$, $M$ and on $r$.

Let us check the H\"older properties of the different elements of the a-priori estimates for linear BSDE with random Lipschitz constant of the Proposition \ref{prop:apriorilinearestimates} by replacing $A,D,C,A',D',C'$ by their counterparts in \eqref{eq:ap:proof:path:01}. 

Firstly, we have
\begin{equation*}
	E\left[ \left( \int_{0}^{T}\abs{\delta A_s+U'_s\delta D_s}ds \right)^{2pq^2} \right] \leq C\left(E\left[ \left( \int_{0}^{T}\abs{\delta A_s}ds \right)^{2pq^2} \right]+ E\left[ \left( \int_{0}^{T}\abs{U'_s\delta D_s}ds \right)^{2pq^2} \right]\right).
\end{equation*}
With Hypothesis (PD b-iv) we get
\begin{equation}\label{eq:nopdb4}
	E\left[ \left( \int_{0}^{T}\abs{\delta A_s}ds \right)^{2pq^2} \right] \leq C\left( \abs{\delta\gamma}^{2\alpha pq^2} +E\left[\left(\int_{0}^{T}\norm{\delta Z_{s}}^2 ds \right)^{2pq^2}\right]\right),
\end{equation}
and  by (PD b-v)
\begin{equation}
	E\left[ \left( \int_{0}^{T}\abs{U'_s\delta D_s}ds \right)^{2pq^2} \right] \leq C\left( E\left[ \left( \sup_{0\leq t \leq T}|U'_{t}|^{2pq^2}\right)\left( \int_{0}^{T} \abs{\delta\gamma}^{\alpha } +\norm{\delta Z_{s}}^{2\alpha_K}ds \right)^{2pq^2}\right]\right).
	\label{eq:ap:proof:path:02}
\end{equation}
Now choose $\bar p$ such that $\bar p  \alpha_{K}<1$, then with $\bar q$ the conjugate exponent of $\bar p$ we have
\begin{equation*}
 E\left[ \left( \sup_{0\leq t \leq T}|U'_{t}|^{2pq^2\bar q}\right)\right]<\infty.
\end{equation*}
Indeed, by Estimate \eqref{eq:momentestimates01} in Proposition \ref{prop:momentestimates}, Equation \eqref{eq:ap:proof:path:LBSDE} and \eqref{eq:ap:proof:path:01} it follows
\begin{equation*}
 E\left[ \left( \sup_{0\leq t \leq T}|U'_{t}|^{2pq^2\bar q}\right)\right] \leq  C E\left[ \abs{\partial_{\gamma}X\left( \gamma' \right)}^{2pq^4\bar q}+\left( \int_{0}^{T}\abs{\partial_{\gamma}f\Big( s,\gamma',Y_{s}\left( \gamma' \right),Z_{s}\left( \gamma' \right)\Big)}ds \right)^{2pq^4\bar q} \right]^{\frac{1}{q^2}},
\end{equation*}
which can be estimated as finite by (D-iv), \eqref{eq:ap:inter01} and (PD b-ii). Hence, \eqref{eq:ap:proof:path:02} becomes
\begin{equation*}
\begin{split}
	E\left[ \left( \int_{0}^{T}\abs{U'_s\delta D_s}ds \right)^{2pq^2} \right]& \leq C\left( \abs{\delta\gamma}^{2\alpha pq^2 } + E\left[\left( \int_{0}^{T}\norm{\delta Z_{s}}^{2\alpha_K}ds \right)^{2pq^2\bar p}\right]\right)\\
					& \leq C\left( \abs{\delta\gamma}^{2\alpha pq^2 } + E\left[\left( \int_{0}^{T}\norm{\delta Z_{s}}^{2}ds \right)^{2pq^2}\right]\right),
	\label{}
\end{split}
\end{equation*}
which in turn implies
\begin{equation}
		E\left[ \left( \int_{0}^{T}\abs{\delta A_s+U'_s\delta D_s}ds \right)^{2pq^2} \right]\leq  C\left( \abs{\delta\gamma}^{2\alpha pq^2 } + E\left[\left( \int_{0}^{T}\norm{\delta Z_{s}}^{2}ds \right)^{2pq^2}\right]\right).
	\label{eq:hoelder01}
\end{equation}
Applying the a priori estimates of Proposition \ref{prop:aprioriestimates}, (PD b-i) and (PD b-0) allows us to estimate the right hand side of the previous inequality as
\begin{equation}
	\begin{split}
		E\left[ \left( \int_{0}^{T}\norm{\delta Z_s}^2ds \right)^{2pq^2} \right]^{(q')^2}&\leq C \abs{\delta \gamma}^{\alpha 4 pq^2 \left( q' \right)^2}+CE\left[ \left(\int_{0}^{T}\abs{\delta f\left( s, Y'_s, Z'_s \right)} ds\right)^{4pq^2 \left( q' \right)^2}\right]\\
		&\leq C_4 \abs{\delta \gamma}^{\alpha 4 pq^2 \left( q' \right)^2}+C \abs{\delta{\gamma}}^{4\alpha pq^2 \left( q' \right)^2}\\
	&\leq C \abs{\delta \gamma}^{\alpha 4 pq^2 \left( q' \right)^2}.
	\end{split}
		\label{eq:hoelder03}
\end{equation}
Hence, \eqref{eq:hoelder01} becomes
\begin{equation}
	E\left[ \left( \int_{0}^{T}\abs{\delta A_s+U'_s\delta D_sds} \right)^{2pq^2} \right]\leq C \left(\abs{\delta\gamma}^{\alpha 2pq^2} + \abs{\delta\gamma}^{4\alpha pq^2}\right) .
	\label{eq:hoelder02}
\end{equation}

Now we consider the last element in Estimate \eqref{eq:apriorilinearestimates}. From \eqref{eq:ap:proof:path:01} and (PD b-vi) we obtain
\begin{equation}
	\begin{split}
		E\left[ \left( \int_{0}^{T}\norm{\delta C_s}^2 ds \right)^{2pq^2} \right] &=E\left[ \left( \int_{0}^{T}\norm{\partial_z f\left( s,\gamma,Y_s,Z_s \right)-\partial_{z}f\left( s,\gamma',Y_s',Z_s' \right)}^2 ds \right)^{2pq^2} \right]\\
		&\leq C\abs{\delta \gamma}^{4\alpha p q^2 }+ CE\left[ \left( \int_{0}^{T}\norm{\delta Z_s}^2ds \right)^{2pq^2} \right].
\end{split}
	\label{eq:hoelder06}
\end{equation}
Inequality \eqref{eq:hoelder03} yields:
\begin{equation}
	\begin{split}
		E\left[ \left( \int_{0}^{T}\norm{\delta C_s}^2 ds \right)^{2pq^2} \right]^{\frac{1}{2q^2}}&\leq C\abs{\delta \gamma}^{2\alpha p }.
\end{split}
	\label{eq:hoelder04}
\end{equation}

For the remaining terms in Inequality \eqref{eq:apriorilinearestimates} note that
$$\sup_{\gamma \in K}E\left[ \abs{\partial_{\gamma}X\left( \gamma \right)}^{2pq^2}+\left(\int_{0}^{T}\abs{A_s\left( \gamma \right)}ds\right)^{2pq^2} \right]^{\frac{1}{2q^2}},$$
due to (PD b-ii), (D-iv) and the boundedness of the BMO norm of $Z$, is a finite constant depending only on $p$, $T$, $K$, $M$, and $r$. Moreover, by (PD b-iii) we have
\begin{equation}
	E\left[ \abs{\delta\partial_{\gamma}X(\gamma)}^{2p} \right]<C(\abs{\delta\gamma}^{2p\alpha})	.
	\label{eq:hoelder05}
\end{equation}

Therefore, taking Inequalities \eqref{eq:hoelder02}, \eqref{eq:hoelder04} and \eqref{eq:hoelder05} together with Inequality \eqref{eq:apriorilinearestimates} we reach:
\begin{equation*}
	\begin{split}
		\norm{U-U'}_{\mathcal{M}^{2p}}^{2p}& \leq CE\left[ \sup_{t \in \left[ 0,T \right]}\abs{\delta U}^{2p} \right]\\
	&\leq C\left( \abs{\delta \gamma}^{2\alpha pq^2}+  \abs{\delta\gamma}^{4\alpha pq^2} \right)^{\frac{1}{q^2}}.
\end{split}
	\label{}
\end{equation*}

Hence we get:
\begin{equation*}
	\norm{U-U'}_{\mathcal{M}^{2p}}\leq C_{16}\abs{\gamma-\gamma'}^{\alpha}.
	\label{}
\end{equation*}
We get then that for each $p>2$, the map $\gamma \mapsto Y\left( \gamma \right)$ from $\mathcal{O}\subset \R^n$ to $\mathcal{M}^p$ is H\"older continuous of order $\alpha$ which prove the penultimate assertion of the theorem.

Now, using lemma 1 page 46 in \cite{sznitman01} by \textsc{Sznitman A.S.}\footnote{The proof of the lemma is based upon a generalization of Kolmogorov's lemma} we have that $\gamma \mapsto Y\left( \gamma \right)$ is pathwise differentiable and the derivative is $\nabla_\gamma Y\left( \gamma \right)$ if $1+\alpha>\frac{n}{p}+1$.
But the previous H\"older continuity holds for any $p>2$, hence it is enough to have a parameter $\alpha>0$ to get the path wise continuity and this ends the proof.
\end{proof}

As already hinted at in Remark \ref{rem:pd:entropic} the generator considered in Section ?? does not fulfill certain assumptions of Theorem \ref{thm:differentiabilityBSDE}. These are in particular the Conditions (PD b-0), (PD b-iv) and (PD b-vi). However, the following corollary shows that Theorem \ref{thm:differentiabilityBSDE} is still valid.
\begin{cor}\label{cor:pd:entropic}
The result of Theorem \ref{thm:differentiabilityBSDE} holds also for $f$ given by
\begin{equation*}
f(s,\gamma,z) = \frac{\gamma}{2}z_2^2-\theta_s z_1-\frac{1}{2\gamma}\theta_s^2.
\end{equation*}
\end{cor}
\begin{proof}
{\it (PD b-0)} An inspection of the proof of Theorem \ref{thm:differentiabilityBSDE} reveals that Condition (PD b-0) is used only in Inequality \eqref{eq:hoelder03}. Note that $|f(s,\gamma,z')-f(s,\gamma',z')|=\frac{1}{2}(z'_2)^2\theta_s^2(\gamma-\gamma')-\frac{1}{2}\theta_s\frac{1}{\gamma\gamma'}(\gamma-\gamma')$. Hence, due to boundedness of $\theta$ and the fact that Estimate \ref{eq:ap:inter01} holds over all $\gamma\in K$, i.e. there exists a $C>0$ such that 
	\begin{equation*}
		\sup_{\gamma\in K}\norm{\left( \int_{0}^{T}\norm{Z_{s}(\gamma)}^2 ds \right)^{\frac{1}{2}}}_{p}\leq C,
	\end{equation*}
the Inequality \eqref{eq:hoelder03} remains true.

{\it (PD b-iv)} The only place in the proof of Theorem \ref{thm:differentiabilityBSDE} where Condition (PD b-iv) is used is in Inequality \eqref{eq:nopdb4}. Note that $\partial_{\gamma}f(s,\gamma,z)= \frac{1}{2}z_2^2+\frac{1}{2\gamma^2}\theta_s$. Hence we have
\begin{equation*}
|\partial_{\gamma}f(s,\gamma,z)-\partial_{\gamma}f(s,\gamma',z')|=\frac{1}{2}(z+z')(z-z')+\frac{1}{2}\theta_s\frac{\gamma+\gamma'}{(\gamma\gamma')^2}(\gamma-\gamma'),
\end{equation*}
which entails for \eqref{eq:nopdb4}
\begin{equation*}
E\left[ \left( \int_{0}^{T}\abs{\delta A_s}ds \right)^{2pq^2} \right] \leq C\left(  \abs{\delta\gamma}^{2pq^2} +E\left[\left(\int_{0}^{T}(Z_s+Z'_s)(\delta Z_{s}) ds \right)^{2pq^2}\right] \right).
\end{equation*}
It remains to apply H\"olders inequality twice and to use \eqref{eq:ap:inter01} as above in order to recover Inequality \eqref{eq:nopdb4}.

{\it (PD b-vi)} We only habe to modify Inequality \eqref{eq:hoelder06}. Note that $\nabla_z f(s,\gamma,z)=(\gamma z_2,-\theta_s )^*$. Since we can write $\gamma z_2 - \gamma' z'_2 = \gamma(z-z') + z'(\gamma-\gamma')$ the wished inequality follows by similar arguments as above.
\end{proof}
